# Supplementary material for: Electron-Transfer-Induced Thermal and Thermoelectric Rectification
Source: arXiv:1908.00495 ancillary file (2019-08-01)
Supplement: Supplementary file 1 [file Supplement.pdf]

# Supplemental Material for "Electron-Transfer-Induced Thermal and Thermoelectric Rectification"

Galen T. Craven,[1] Dahai He,[2] and Abraham Nitzan[1,3]

[1]Department of Chemistry, University of Pennsylvania, Philadelphia, PA 19104, USA

[2]Department of Physics and Institute of Theoretical Physics and Astrophysics, Xiamen University, Xiamen 361005, Fujian, China

[3]School of Chemistry, Tel Aviv University, Tel Aviv 69978, Israel

## I. MOLECULE-TO-MOLECULE ELECTRON TRANSFER RATE CONSTANTS FOR POSITIVE AND NEGATIVE THERMAL BIAS STATES

Consider an electron transfer (ET) process between a pair of molecular donor-acceptor sites in the positive and negative thermal bias states (denoted " + " and " − ", respectively) discussed in the main text in which the redox sites are seated in respective environments $A$ and $B$ which have different local temperatures $T_A$ and $T_B$. Specifically, in the positive thermal bias state environments $A$ and $B$ have temperatures $T_A = T - \Delta T/2$ and $T_B = T + \Delta T/2$ and in the negative thermal bias state the temperatures are exchanged ($\Delta T \to -\Delta T$) with $T_A = T + \Delta T/2$ and $T_B = T - \Delta T/2$. The electronic subsystem is coupled to two groups of harmonic vibrational modes, each associated with one of the environments $A$ or $B$, that are in equilibrium at the respective environment temperature. The system has two electronic states, $a$ and $b$, which each represent electron localization on one of the redox sites. A general expression for the thermally-averaged electron transfer rate between donor and acceptor in the corresponding thermal bias state can be written in terms of Fermi's golden rule (FGR) as

$$k^{\pm}_{m\to n} = \frac{2\pi}{\hbar}|V_{mn}|^2 \sum_{\boldsymbol{\nu}} P^{\pm}_{\boldsymbol{\nu}} \sum_{\boldsymbol{\nu}'} \left|\langle \chi_{n,\boldsymbol{\nu}'}|\chi_{m,\boldsymbol{\nu}}\rangle\right|^2 \delta(\hbar\omega_{m,\boldsymbol{\nu}|n,\boldsymbol{\nu}'}), \tag{S1}$$

where $V_{mn}$ is the electronic coupling between states $m \in \{a,b\}$ and $n \in \{a,b\} : n \neq m$ evaluated in the Franck-Condon limit, $\boldsymbol{\nu} = \{\nu_1, \nu_2, \ldots, \nu_N\}$ and $\boldsymbol{\nu}' = \{\nu'_1, \nu'_2, \ldots, \nu'_N\}$ are sets of vibrational quanta for the vibrational modes in electronic states $m$ and $n$, $\chi_{m,\boldsymbol{\nu}}$ and $\chi_{n,\boldsymbol{\nu}'}$ are the vibrational wave functions in each state, and

$$\hbar\omega_{m,\boldsymbol{\nu}|n,\boldsymbol{\nu}'} = \hbar\omega_{mn} + \sum_{j\in A\cup B} \hbar\omega_j \left(\nu'_j - \nu_j\right) \tag{S2}$$

is the energy difference between the two states accounting for both the electronic and vibrational contributions to the total system energy with $\hbar\omega_{mn}$ being the electronic energy difference between

states and $\omega_j$ the frequency of vibrational mode $j$. Equation (S2) is derived using a displaced oscillator approximation in which the frequency of each mode is independent of the electronic state. The probability to observe the system with a specific set of vibrational quanta in the corresponding thermal bias state is

$$
\begin{aligned}
P_{\boldsymbol{\nu}}^{\pm} &= \left(\prod_{j\in A} P_{j\in A,\nu_j}^{\pm}\right)\left(\prod_{j\in B} P_{j\in B,\nu_j}^{\pm}\right) \\
&= \left(\prod_{j\in A} \frac{\exp\left[\hbar\omega_j\left(\nu_j+\frac{1}{2}\right)/k_{\mathrm{B}}T_A\right]}{\sum\limits_{\nu_j\in\boldsymbol{\nu}_j}\exp\left[\hbar\omega_j\left(\nu_j+\frac{1}{2}\right)/k_{\mathrm{B}}T_A\right]}\right)\left(\prod_{j\in B} \frac{\exp\left[\hbar\omega_j\left(\nu_j+\frac{1}{2}\right)/k_{\mathrm{B}}T_B\right]}{\sum\limits_{\nu_j\in\boldsymbol{\nu}_j}\exp\left[\hbar\omega_j\left(\nu_j+\frac{1}{2}\right)/k_{\mathrm{B}}T_B\right]}\right),
\end{aligned}
\tag{S3}
$$

where $P_{j\in E,\nu_j}^{\pm} : E \in \{A, B\}$ is the probability to observe mode $j$ in state $\nu_j$ given that it associated with environment $E$ (this implies that mode $j$ is thermalized at the temperature of environment $E$).

In a particular thermal bias state, Eq. (S1) can be expressed in terms of a corresponding time-correlation function $G_j^{\pm}(t)$ for each mode $j$ [1]:

$$
k_{m\to n}^{\pm} = \frac{|V_{mn}|^2}{\hbar}\int_{\mathbb{R}} dt \exp\left[i\omega_{mn}t\right]\left(\prod_{j\in A} G_j^{\pm}(t)\right)\left(\prod_{j\in B} G_j^{\pm}(t)\right),
\tag{S4}
$$

with

$$
G_j^{\pm}(t) = \sum_{\nu_j\in\boldsymbol{\nu}_j} P_{j\in E,\nu_j}^{\pm} \sum_{\nu_j'\in\boldsymbol{\nu}_j'} \left|\langle\chi_{n,\nu_j'}|\chi_{m,\nu_j}\rangle\right|^2 \exp\left[i\omega_j t\left(\nu_j'-\nu_j\right)\right] : E\in\{A,B\}\,.
\tag{S5}
$$

where $\boldsymbol{\nu}_j$ and $\boldsymbol{\nu}_j'$ denote the sets of vibrational states for mode $j$ in electronic states $m$ and $n$. After applying the methods outlined in Refs. 2 and 3 to reduce $G_j^{\pm}(t)$ to a closed-form expression, the ET rate in the corresponding thermal bias state can be written as

$$
\begin{aligned}
k_{m\to n}^{\pm} = \frac{|V_{mn}|^2}{\hbar^2}\int_{\mathbb{R}} dt \exp\left[i\omega_{mn}t\right] &\exp\left[-\sum_{j\in A} S_j\left(\left(2n_{j,A}^{\pm}+1\right)-\left(n_{j,A}^{\pm}+1\right)e^{i\omega_j t}-n_{j,A}^{\pm}e^{-i\omega_j t}\right)\right] \\
\times &\exp\left[-\sum_{j\in B} S_j\left(\left(2n_{j,B}^{\pm}+1\right)-\left(n_{j,B}^{\pm}+1\right)e^{i\omega_j t}-n_{j,B}^{\pm}e^{-i\omega_j t}\right)\right],
\end{aligned}
\tag{S6}
$$

where

$$
S_j = \frac{E_{\mathrm{R}j}}{\hbar\omega_j},
\tag{S7}
$$

is the Huang-Rhys factor for mode $j$ with $E_{\mathrm{R}j}$ being the reorganization energy of that mode [1] and

$$
n_{j,E}^{\pm} = \frac{1}{\exp\left[\hbar\omega_j/k_{\mathrm{B}}T_E\right]-1} : E\in\{A,B\}\,,
\tag{S8}
$$

is the thermally-averaged phononic population of mode $j$ in the corresponding thermal bias state given that it is associated with environment $E$. Expanding the exponential terms $\exp[\pm i\omega_j t]$ to second order and evaluating the time integrals in Eq. (S6) yields

$$k^{\pm}_{m\to n} = \frac{|V_{mn}|^2}{\hbar^2}\sqrt{\frac{2\pi}{\sum_{j\in A} S_j\omega_j^2\left(2n^{\pm}_{j,A}+1\right)+\sum_{j\in B} S_j\omega_j^2\left(2n^{\pm}_{j,B}+1\right)}} \times \exp\left[-\frac{\left(\omega_{mn}+\sum_j^N S_j\omega_j\right)^2}{2\left(\sum_{j\in A} S_j\omega_j^2\left(2n^{\pm}_{j,A}+1\right)+\sum_{j\in B} S_j\omega_j^2\left(2n^{\pm}_{j,B}+1\right)\right)}\right]. \tag{S9}$$

In the limit where the vibrational energy of each mode that participates in the ET process is small compared the thermal energy of its corresponding environment, the rate constant in (S9) reduces to the Marcus-type form:

$$k^{\pm}_{m\to n} = \frac{|V_{mn}|^2}{\hbar}\sqrt{\frac{\pi}{k_{\rm B}(T_A E_{\rm R}A + T_B E_{\rm R}B)}}\exp\left[-\frac{(\Delta E_{nm}+E_{\rm R})^2}{4k_{\rm B}(T_A E_{\rm R}A + T_B E_{\rm R}B)}\right], \tag{S10}$$

where $E_{\rm R}A = \sum_{j\in A} E_{{\rm R}j}$ and $E_{\rm R}B = \sum_{j\in B} E_{{\rm R}j}$.

In the single-temperature limit, the model described above is equivalent to the standard polaron model with $\hat{H}_{\text{e-ph}} = \sum_{j,s} C_j^{(s)}\hat{c}_s^\dagger\hat{c}_s(\hat{a}_j+\hat{a}_j^\dagger)$ where $\hat{c}_s^\dagger(\hat{c}_s)$ are creation (annihilation) operators for the electron on the molecular site in environment $s\in\{A,B\}$ at energy $\epsilon_s$, $\hat{a}_j^\dagger(\hat{a}_j)$ are similar operators for phonons in mode $j$ of energy $\hbar\omega_j$, and $C_j^{(s)}$ is the electron-phonon coupling of mode $j$ defined by the relation $E_{{\rm R}j} = |C_j^{(s)}|^2/\hbar\omega_j$.

## II. THERMALLY-HOMOGENEOUS MOLECULE-TO-METAL ELECTRON TRANSFER RATE CONSTANTS

In the two-site molecular junction model considered in the main text, the electron transfer rates at the thermally - homogeneous (that is, single temperature) molecule-metal interfaces for the corresponding thermal bias state across the junction are given by the respective Marcus forms [1, 4]:

$$k^{\pm}_{a\to M} = \sqrt{\frac{1}{4\pi k_{\rm B}T_A E_{\rm R}A}}\int_{\mathbb{R}}\left[1-f\left(T_A,\mu_A,\epsilon\right)\right]\Gamma_A(\epsilon)\exp\left[-\frac{\left(\Delta E_{M_A}+\epsilon+E_{\rm R}A\right)^2}{4k_{\rm B}T_A E_{\rm R}A}\right]d\epsilon, \tag{S11}$$

$$k^{\pm}_{M\to a} = \sqrt{\frac{1}{4\pi k_{\rm B}T_A E_{\rm R}A}}\int_{\mathbb{R}} f\left(T_A,\mu_A,\epsilon\right)\Gamma_A(\epsilon)\exp\left[-\frac{\left(-\Delta E_{M_A}-\epsilon+E_{\rm R}A\right)^2}{4k_{\rm B}T_A E_{\rm R}A}\right]d\epsilon, \tag{S12}$$

$$k^{\pm}_{b\to M} = \sqrt{\frac{1}{4\pi k_{\rm B}T_B E_{\rm R}B}}\int_{\mathbb{R}}\left[1-f\left(T_B,\mu_B,\epsilon\right)\right]\Gamma_B(\epsilon)\exp\left[-\frac{\left(\Delta E_{M_B}+\epsilon+E_{\rm R}B\right)^2}{4k_{\rm B}T_B E_{\rm R}B}\right]d\epsilon, \tag{S13}$$

$$k^{\pm}_{M\to b} = \sqrt{\frac{1}{4\pi k_{\rm B}T_B E_{\rm R}B}}\int_{\mathbb{R}} f\left(T_B,\mu_B,\epsilon\right)\Gamma_B(\epsilon)\exp\left[-\frac{\left(-\Delta E_{M_B}-\epsilon+E_{\rm R}B\right)^2}{4k_{\rm B}T_B E_{\rm R}B}\right]d\epsilon, \tag{S14}$$

where $f(T,\mu,\epsilon) = (\exp[(\epsilon-\mu)k_{\mathrm{B}}T]+1)^{-1}$ is a Fermi-Dirac distribution, and

$$\Gamma_E(\epsilon) = \left(\frac{2\pi}{\hbar}|V_E|^2\rho_E\right)_\epsilon, \tag{S15}$$

is the molecule-metal coupling at electrode $M_E : E \in \{A, B\}$ with $\rho_E$ and $V_E$ being, respectively, the single electron density of states and the coupling between energy surfaces at the corresponding interface, both of which are functions of $\epsilon$. Without loss of generality, we take $\mu = 0$ in all calculations. Note that in the main text the wide-band approximation is applied to describe the electronic structure of the metals, and thus $\Gamma_A$ and $\Gamma_B$ are taken to be constant. Specifically, $\Gamma_A = \Gamma_B = 100\,\mathrm{ps}^{-1}$ in all calculations. The reaction free energy for ET from molecule to metal at the corresponding interface is $\Delta E_{M_E}$ with $\Delta E_{M_A} - \Delta E_{M_B} = \Delta E_{ba}$.

## III. HEAT CURRENT DERIVATION

The electron-transfer-induced heat current between the molecular donor and acceptor environments $A$ and $B$ discussed in the main text is generated by the electron-phonon interaction of each vibrational mode that participates in the ET process. Consider the energy change in each environment during an ET event. With nuclear tunneling disregarded, ET is dominated by configurations of modes $\boldsymbol{x} = (x_1, x_2, \ldots, x_N)$ where the two electronic states $a$ and $b$ have equal energy. This is a criterion that arises from the physical constraint that energy is conserved during the transition between states. The mode configurations where this energy-conserving ET process can occur are defined by the transition surface (TS):

$$\boldsymbol{x}^\ddagger = \{\boldsymbol{x} : E_a(\boldsymbol{x}) = E_b(\boldsymbol{x})\}, \tag{S16}$$

which is the set of points where the energy surfaces $E_a$ and $E_b$ have equal energy; electron transfer can occur at any point $\boldsymbol{x} \in \boldsymbol{x}^\ddagger$ and thus this must be accounted for in the calculations that follow. Consider the energy change $\mathcal{Q}_j$ in mode $j$ during the $m \to n$ transition. The total energy change contributed by mode $j$ in the environment ($A$ or $B$) of which $j$ is an element is the sum of energy released by the environment during the ascent to the TS on the $E_m$ surface and the energy obtained by the environment during the descent to equilibrium from the TS on the $E_n$ surface

$$\mathcal{Q}_j^{(m\to n)} \equiv -\mathcal{Q}_{\mathrm{rel}}^{(m)} + \mathcal{Q}_{\mathrm{obt}}^{(n)}. \tag{S17}$$

For the $m \to n$ transition the amount of heat transferred by mode $j$ into the environment $A$ or $B$ given that $j$ is an element of that particular environment is

$$\begin{aligned} \mathcal{Q}_j^{(m\to n)} &= -\mathcal{Q}_j^{(n\to m)} \\ &\equiv -\frac{1}{2}\kappa_j \left(x_j - \lambda_j^{(m)}\right)^2 + \frac{1}{2}\kappa_j \left(x_j - \lambda_j^{(n)}\right)^2 . \end{aligned} \tag{S18}$$

For simplicity, we have taken the signs in (S18) so that $\mathcal{Q}$ is positive when energy is obtained by the corresponding environment and negative when energy is released by corresponding environment. During the electronic state transition $m \to n$, the expectation value for the amount of heat released to/obtained from the environment ($A$ or $B$) that contains mode $j$ is given by

$$\left\langle \mathcal{Q}_j^{(m\to n)} \right\rangle^{\pm} = \int_{\mathbb{R}^N} \mathcal{Q}_j^{(m\to n)}(\boldsymbol{x})\, P^{\ddagger}_{m\to n}(\boldsymbol{x}, \pm)\, dx_1 \ldots dx_N, \tag{S19}$$

where $P^{\ddagger}_{m\to n}(\boldsymbol{x}, \pm)$ is the conditional probability density in the corresponding thermal bias state that ET occurs through a specific point on the TS given that the configuration of modes $\boldsymbol{x}$ is on the TS. In the classical limit, the conditional probability densities on the TS for the respective thermal bias states are

$$P^{\ddagger}_{m\to n}(\boldsymbol{x}, \pm) = \frac{\delta\Big(E_n(\boldsymbol{x}) - E_m(\boldsymbol{x})\Big) \prod_{j\in A} \exp\left[\dfrac{-\frac{1}{2}\kappa_j \left(x_j - \lambda_j^{(m)}\right)^2}{k_{\mathrm{B}} T_A}\right] \prod_{j\in B} \exp\left[\dfrac{-\frac{1}{2}\kappa_j \left(x_j - \lambda_j^{(m)}\right)^2}{k_{\mathrm{B}} T_B}\right]}{\int_{\mathbb{R}^N} \delta\Big(E_n(\boldsymbol{x}) - E_m(\boldsymbol{x})\Big) \prod_{j\in A} \exp\left[\dfrac{-\frac{1}{2}\kappa_j \left(x_j - \lambda_j^{(m)}\right)^2}{k_{\mathrm{B}} T_A}\right] \prod_{j\in B} \exp\left[\dfrac{-\frac{1}{2}\kappa_j \left(x_j - \lambda_j^{(m)}\right)^2}{k_{\mathrm{B}} T_B}\right] dx_1 \ldots dx_N}, \tag{S20}$$

where the $\delta$-function constrains the system to mode configurations where $E_m(\boldsymbol{x}) = E_n(\boldsymbol{x})$. Evaluation of (S19) coupled with (S20) can be accomplished using the methods developed in Ref. 5.

The general form for the steady state electron-transfer-induced heat current between environments $A$ and $B$ in the corresponding thermal bias state under the system conditions at which the net electronic flux vanishes is [6]:

$$\begin{aligned} \mathcal{J}_{\mathcal{Q}}^{\pm} &= \mathcal{J}_{\mathrm{el}}^{\pm} \left( \left\langle \mathcal{Q}_j^{(m\to n)} \right\rangle^{\pm} + \left\langle \mathcal{Q}_j^{(n\to m)} \right\rangle^{\pm} \right) \\ &= \mathcal{J}_{\mathrm{el}}^{\pm} \frac{2(T_B - T_A) E_{\mathrm{R}A} E_{\mathrm{R}B}}{T_A E_{\mathrm{RA}} + T_B E_{\mathrm{R}B}}, \end{aligned} \tag{S21}$$

where $\mathcal{J}_{\mathrm{el}}^{\pm}$ is the unidirectional electron flux between sites. Examples for the particular systems considered in the main text are given below.

### A. Electron-Transfer-Induced Heat Current Between Molecules

In the case of the first system considered in the main text which consists of two molecular sites only, the steady state electron flux is

$$\mathcal{J}_{\mathrm{el}}^{\pm} = \frac{k_{a\to b}^{\pm} k_{b\to a}^{\pm}}{k_{a\to b}^{\pm} + k_{b\to a}^{\pm}}, \tag{S22}$$

which can be substituted into (S21) to obtain the corresponding heat current.

### B. Electron-Transfer-Induced Heat Current in a Molecular Junction

For the metal-molecule-molecule-metal junction considered in the main text, the unidirectional steady state electron flux between molecular charge transfer sites in the $A \to B$ and reverse $B \to A$ directions are, respectively,

$$\begin{aligned} \mathcal{J}_{a\to b}^{\pm} = k_{a\to b}^{\pm}\Big(&k_{b\to a}^{\pm} k_{M\to a}^{\pm} + k_{b\to M}^{\pm} k_{M\to a}^{\pm} + k_{b\to a}^{\pm} k_{M\to b}^{\pm}\Big) \\ \Big/\Big(&\big(k_{b\to a}^{\pm} + k_{b\to M}^{\pm}\big)\big(k_{a\to M}^{\pm} + k_{M\to a}^{\pm}\big) \\ &+ \big(k_{a\to M}^{\pm} + k_{b\to a}^{\pm}\big) k_{M\to b}^{\pm} \\ &+ \big(k_{b\to M}^{\pm} + k_{M\to a}^{\pm} + k_{M\to b}^{\pm}\big) k_{a\to b}^{\pm}\Big), \end{aligned} \tag{S23}$$

$$\begin{aligned} \mathcal{J}_{b\to a}^{\pm} = k_{b\to a}^{\pm}\Big(&k_{a\to b}^{\pm} k_{M\to a}^{\pm} + k_{a\to M}^{\pm} k_{M\to b}^{\pm} + k_{a\to b}^{\pm} k_{M\to b}^{\pm}\Big) \\ \Big/\Big(&\big(k_{b\to a}^{\pm} + k_{b\to M}^{\pm}\big)\big(k_{a\to M}^{\pm} + k_{M\to a}^{\pm}\big) \\ &+ \big(k_{a\to M}^{\pm} + k_{b\to a}^{\pm}\big) k_{M\to b}^{\pm} \\ &+ \big(k_{b\to M}^{\pm} + k_{M\to a}^{\pm} + k_{M\to b}^{\pm}\big) k_{a\to b}^{\pm}\Big). \end{aligned} \tag{S24}$$

In the heat currents reported in the main text these electron fluxes are calculated under the condition of zero electronic current $\Rightarrow \mathcal{J}_{\mathrm{el}}^{\pm} \equiv \mathcal{J}_{\mathrm{el}}^{\pm}\big|_{I^{\pm}=0} = \mathcal{J}_{a\to b}^{\pm} = \mathcal{J}_{b\to a}^{\pm}$ where

$$\begin{aligned} \frac{I^{\pm}}{e} = \Big(&k_{a\to M}^{\pm} k_{b\to a}^{\pm} k_{M\to b}^{\pm} - k_{M\to a}^{\pm} k_{a\to b}^{\pm} k_{b\to M}^{\pm}\Big) \\ \Big/\Big(&\big(k_{b\to a}^{\pm} + k_{b\to M}^{\pm}\big)\big(k_{a\to M}^{\pm} + k_{M\to a}^{\pm}\big) \\ &+ \big(k_{a\to M}^{\pm} + k_{b\to a}^{\pm}\big) k_{M\to b}^{\pm} \\ &+ \big(k_{b\to M}^{\pm} + k_{M\to a}^{\pm} + k_{M\to b}^{\pm}\big) k_{a\to b}^{\pm}\Big), \end{aligned} \tag{S25}$$

is the electronic current through the junction. The zero current electron flux $\mathcal{J}_{\mathrm{el}}^{\pm}\big|_{I^{\pm}=0}$ is then used in (S21) to obtain the corresponding heat current.

### C. Electronic Current in the Coherent Limit

The electronic current generated in the two-level ($E'_a$ and $E'_b$) molecular bridge examined in the main text can be derived in the coherent limit of transport where there is no vibronic coupling using the Landauer expression [1]:

$$I(\Phi, T_A, T_B) = \frac{e}{\pi\hbar}\int_{-\infty}^{\infty} \mathcal{T}(\epsilon)\Big[f(T_B, \mu_B(\Phi), \epsilon) - f(T_A, \mu_A(\Phi), \epsilon)\Big]d\epsilon, \tag{S26}$$

where

$$\mathcal{T}(\epsilon) = \mathrm{Tr}\left[\hat{\Gamma}_A(\epsilon)\hat{G}^\dagger(\epsilon)\hat{\Gamma}_B(\epsilon)\hat{G}(\epsilon)\right], \tag{S27}$$

is the transmission coefficient with

$$\hat{\Gamma}_A(\epsilon) = \begin{pmatrix} \hbar\Gamma_A(\epsilon) & 0 \\ 0 & 0 \end{pmatrix} \qquad \text{and} \qquad \hat{\Gamma}_B(\epsilon) = \begin{pmatrix} 0 & 0 \\ 0 & \hbar\Gamma_B(\epsilon) \end{pmatrix} \tag{S28}$$

being the respective matrices that couple each level to the corresponding electrode with which it interacts, and $\hat{G}(\epsilon)$ is a Green's function, with conjugate adjoint $\hat{G}^\dagger(\epsilon)$, that is defined by

$$\hat{G}^{-1}(\epsilon) = \begin{pmatrix} \epsilon - E'_a + \frac{1}{2}i\hbar\Gamma_A(\epsilon) & V_{ab} \\ V_{ba} & \epsilon - E'_b + \frac{1}{2}i\hbar\Gamma_B(\epsilon) \end{pmatrix}. \tag{S29}$$

Evaluating (S27) in the wide-band limit we obtain

$$\mathcal{T}(\epsilon) = \frac{|V_{ab}|^2\hbar^2\Gamma_A\Gamma_B}{\left|\left(\epsilon - E'_a + \frac{1}{2}i\hbar\Gamma_A\right)\left(\epsilon - E'_b + \frac{1}{2}i\hbar\Gamma_B\right) - |V_{ab}|^2\right|^2}, \tag{S30}$$

for the transmission coefficient. To obtain the coherent thermoelectric results shown in the main text (see Fig. 5), the equation $I(\Phi, T_A, T_B) = 0$ is solved numerically to obtain the voltage bias $\Phi$ that gives zero current for a specific temperature bias $\Delta T = T_B - T_A$.

---

[1] A. Nitzan, *Chemical Dynamics in Condensed Phases: Relaxation, Transfer, and Reactions in Condensed Molecular Systems* (Oxford University Press, 2006).

[2] S. H. Lin, J. Chem. Phys. **44**, 3759 (1966), doi:10.1063/1.1726531.

[3] S. H. Lin, C. H. Chang, K. K. Liang, R. Chang, Y. J. Shiu, J. M. Zhang, T.-S. Yang, M. Hayashi, and F. C. Hsu, Adv. Chem. Phys. **121**, 1 (2002), doi:10.1002/0471264318.ch1.

[4] R. A. Marcus, J. Chem. Phys. **43**, 679 (1965), doi:10.1063/1.1696792.

[5] G. T. Craven and A. Nitzan, Phys. Rev. Lett. **118**, 207201 (2017), doi:10.1103/PhysRevLett.118.207201.

[6] G. T. Craven and A. Nitzan, Proc. Natl. Acad. Sci. **113**, 9421 (2016), doi:10.1073/pnas.1609141113.
